# Supplementary material for: On-Device CPU Scheduling for Sense-React Systems
Source: arXiv:2207.13280 source file (2022-08-14)
Supplement: Supplementary file 1 [file appendix.tex]

We will describe our theoretical formulation in more detail here.

\section{Stage I: Core Allocation}
For a DAG with $n$ subchains on a system with $k$ cores, \oursys' first stage of optimization outputs a boolean matrix of size $n \times k$, where an element $a_{ij}$ is 1 if subchain $i$ is allowed to execute on core $j$. 
We use $c_x$ to denote the computation time of node x, and $x \in SC_i$ is the set of all nodes which belong to subchain i.

Let C denote the number of chains in the DAG. We denote by $l_c$ and $t_c$ the latency and period (i.e. reciprocal of throughput) along a chain, and by $p_s$ the period of subchain s, and by $|c|$ the length of chain c. M denotes a very large number (we use 50,000 in our implementation).

% \vspace{-1em}
\setcounter{equation}{0}
\begin{align}
\text{min} & \sum_{c=1}^{C} (w_{1c} * l_c + w_{2c} * t_c) + \sum_{s=1}^{n} w_{3s} * p_s &  \\
\text{s.t.} \sum_{j=1}^k a_{ij} & \geq 1.0 & \forall i \\
 \sum_{i=1}^n a_{ij} & \geq 1.0 & \forall j \\
 \sum_{j=1}^k a_{ij} & \geq 1.0 - M*( 1 - x_i) & \forall i \\
 \sum_{j=1}^k a_{ij} & \leq 1.0 + M*x_i & \forall i \\ 
 y_{ij} & \leq a_{ij} & \forall i,j \\
 y_{ij} & \leq x_{i} & \forall i,j \\
 y_{ij} & \geq x_i + a_{ij} - 1 & \forall i,j \\
 \sum_{i=1}^n a_{ij} & \leq 1 + M(1 - y_{ij}) & \forall i,j \\
 \sum_{i=1}^n a_{ij} & \geq 1 - M(1 - y_{ij}) & \forall i,j \\
 z_{ij} & \leq M(a_{ij}) & \forall i,j \\
 z_{ij} & \leq p_i & \forall i,j \\
 p_i - z_{ij} & \leq M(1 - a_{ij}) & \forall i,j \\
 \sum_{j=1}^{k} z_{ij} & \geq (max_{x \in SC_i} c_x)*b_i & \forall i \\
 1 - Mx_i & \leq b_i \leq 1 + Mx_i & \forall i \\
 \sum_{j=1}^{k} z_{ij} & \geq \sum_{x \in SC_i} c_x & \forall i \\
 w_{ijl} & \leq a_{ij} & \forall i,j,l
\end{align}

\begin{align}
w_{ijl} & \leq a_{lj} & \forall i,j,l \\
 w_{ijl} & \geq a_{ij} + a_{lj} - 1.0 & \forall i,j,l \\
 p_i & \geq (\sum_{x \in SC_i} c_x) * (\sum_{l=1}^{n} \sum_{j=1}^{k} w_{ijl}) - Mx_i & \forall i \\
\text{if not $P_i$ : } b_i & = \sum_{j=1}^{k} a_{ij}  & \forall i \\
 ex_i & \geq p_i - Mx_i & \forall i \\
 ex_i & \geq \sum_{x \in SC_i} c_x & \forall i
\end{align}

Equation 5.1 represents the objective function, which is a weighted linear sum of the low level metrics. The parameters $w_{1c} \& w_{2c}$ represent the weights for the latency and period of chain c respectively. $w_{3s}$ represents the weight for the period of subchain s. 

Eqn. 5.2 and 5.3 represent that each subchain (core) should be assigned at least one core (subchain) respectively.

$x_i$ denotes whether a subchain gets more than one cores, and Eqn 5.4 and 5.5 represent this. Equations 5.6 - 5.8 enforce that $y_{ij} = a_{ij} \&\& x_i$, since $y_{ij}$ represents whether subchain i is on multiple cores ($x_i$) and core j is one of them ($a_{ij}$). Equations 5.9 - 5.10 denote that if $y_{ij} = 1$, then there should be only one subchain on core j. All these eqns together enforce our assumption A1.

We analytically lower bound the period of each subchain based on the $a_{ij}$ parameters. Lets take two cases:

\paragraphi{Case 1} If a subchain gets $\sum_{j=1}^{k} a_{ij}$ cores to execute, then $q_i = \frac{\sum_{j=1}^k a_{ij} }{b_i}$ would be the degree of parallelism i.e.  we allow each node in the subchain to use at most $q$ cores. As per approximation Ap2, we assume each node's computation time scales perfectly with q [which we forgo in \S\ref{sec:singlecore}], and and the period is given by $p_i = max(max_{x \in SC_i} (c_x / q_i), \Sigma_{x \in SC_i} (c_x)/b_i)$. This formula was inspired by our theoretical result of optimal response time for a single chain on multiple cores, explained in more detail in \S\ref{sec:singlecore}. We encode this formula (eqn 5.14, 5.16) in our formulation by making extra variables $z_{ij} = p_{i}a_{ij}$ (Eqns 5.11 - 5.13). Eqn 5.15 signifies that $q_i = b_i = 1$ if the subchain is on a single core, eqn 21 states that $q_i = 1$ and consequently $b_i$ is the number of cores alloted to the subchain, if it is not parallelizable. The MILP solver will make the trade off of $q_i$ while solving for $a_{ij}$; a larger $q_i$ may reduce per-node processing times, but also reduces the degree of pipelining along the subchain. Note that we didn't directly use the $q_i$ parameter in our constraints so as to be able to linearize the formulation.

\paragraphi{Case 2} If a core has $s = \sum_{i=1}^{n} a_{ij}$ subchains assigned, then, due to approximation Ap1, each subchain i gets $1/s$ share of the CPU, and hence will finish one execution in time $(\sum_{x \in SC_i} c_x) * s$. This is represented in eqn 5.20, where in, if subchain i doesn't have $>1$ cores, we lower bound the chain's period by the product of the computation time of the subchain multiplied to the total number of subchains on its core. To help express this constraint in a linear form, we make extra variables of the form $w_{ijl}$, which represent if subchain i and l share core j [represented in Eqns 5.17 - 5.19]. Note that we forgo this approximation in \S\ref{sec:singlecore}, wherein we design a fine grained scheduling policy for each such core.

The variable $ex_i$ represents the execution time of a subchain i, i.e. how long does it take to finish one full execution \& produce an output. It is at least the total computation time of the subchain (eqn 5.23), and is equal to the subchain's period if it is on a single core (eqn. 5.24) [one could get a tighter bound but we use this approximation].

Let chain c be denoted by $s_{c0}, s_{c1}..$. Eqn 5.24 and 5.27 describe the chain throughput and latency as a function of other variables. We add constraints corresponding to the following : $LT_x$ ($LT_c$) and $UT_x$ ($UT_c$) represent the lower and upper bounds on the throughput of node x (chain c) respectively. $LL_c$ and $UL_c$ similarly represent the lower and upper bound constraints on the chain c's latency. We can also add constraints/ weights on the chain's response time, which we approximate as $l_c + t_c$. Eqns 5.25, 5.26 and 5.28 represent these constraints.
\vspace{-0.1em}
\begin{align}
t_c & \geq p_i & \forall SC_i \in C_c \\
LT_c & \leq t_c \leq UT_c & \forall c \\
LT_x & \leq p_i \leq UT_x & \forall x \in SC_i \\
l_c & \geq ex_{c0} + \sum_{r=1}^{|c|} ex_{cr} + p_{cr} & \forall c \\
LL_c & \leq l_c \leq UL_c & \forall c
\end{align}

\section{Stage II: Per Core \& Per Subchain Scheduling}
Given the subchain to core mappings from our first optimization stage, the next stage makes finer-grained scheduling decisions for each subchain and core. There are two distinct cases to consider: 

\paragraphb{Single subchain on one or more cores} We shall now extend the approach mentioned in \S\ref{sec:multicore} (Case 1). Considering a subchain of nodes $\{n_1, n_2, \ldots n_m\}$ with $k$ assigned cores. The scheduler must determine the rate (or the time period $p$) of the source node ($n_1$) and the degree of parallelism for each node, such that the response time is minimized. We allow each node in the subchain to use at most $q$ cores (only a subset may be designed to use all $q$), and set $p = max(max_{j=1}^m (c^q_j), \Sigma_{j=1}^{m} (c^q_j)/\lfloor k/q \rfloor)$, where $c^q_j$ is $n_j$'s computation time with at most $q$ cores \footnote{Note that we are not assuming perfect scaling here, and can use the actual/empirical compute time of each node given q cores}. We have proved that this rate allocation achieves response time (for this particular subchain) within $2 \times$ the optimal, and equal to the optimal for $q = 1$~\cite{supplementary-proofs}. The value of $q$ ranges from $1$ to $k$; a larger $q$ may reduce per-node processing times, but also reduces the degree of pipelining along the subchain. The scheduler iterates over all $k$ choices for this subchain, and selects the value of $q$ that results in lowest response time for this subchain.

\paragraphb{Multiple subchains on a single core} For subchains  $s_1, s_2 ...s_n$ assigned the same core $Q_j$, the scheduler must determine the temporal allocation of CPU time across them. We define a variable $f_i$ for each subchain, which denotes two things: a) the subchain gets $\Sigma_{x \in SC_i} (c_x) * f_i$ CPU time per period, b) the subchain finishes one execution per $1/f_i$ periods. The total period of this schedule then comes out to be $\sum_{i \in C_j} f_i * (\Sigma_{x \in SC_i} (c_x))$. The execution of each (fractional) subchain within a period follows topological ordering. Such a schedule ensures that the CPU core is fully-utilized, while the fraction variables tune the core allocation across subchains. We distinguish between subchains (or nodes) which have constraints on average throughput (e.g. streaming nature such as GML) from others, by allowing f to take arbitrary values for such nodes, but constraining it to be integral - reciprocal (i.e. $1/f_i$ is an integer) for other nodes. This is because, $1/f_i$ being integral allows the scheduler to control the exact throughput of the subchain.

We approximate the per chain metrics as an analytical function of these fraction variables, and formulate a Geometric Programming problem to compute these variables such that the specified objective function is optimized. We now describe our formulation. Note that we make a single GP problem to solve for temporal CPU allocation of all the cores. Let SN denote the set of subchains of the streaming nature, and let $Q_j$ denote core j, and $SQ_j$ denote the set of all the subchains sharing core j. 
\vspace{-0.05em}
\begin{align}
\text{min} & \sum_{c=1}^{C} (w_{1c} * l_c + w_{2c} * t_c) + \sum_{s=1}^{n} w_{3s} * p_s &  \\
\text{s.t.} f_i & \leq 1.0 & \forall x \notin \text{SN} \\
p^q_j & \geq \sum_{i \in SQ_j} (f_i * \Sigma_{x \in SC_i} (c_x) )  & \forall j 
\end{align}
\begin{align}
p_i & \geq \frac{1}{f_i} * p^q_j & \forall i \in SQ_j \\
% f_i * () & \geq 1.0 & \forall i \\
t_c & \geq p_i & \forall SC_i \in C_c \\
LT_x & \leq p_i \leq UT_x & \forall x \in SC_i \\
l_c & \geq p_{c0} + \sum_{r=1}^{|c|} 2*p_{cr} & \forall c \\
LT_c & \leq t_c \leq UT_c & \forall c \\
LL_c & \leq l_c \leq UL_c & \forall c
\end{align}
\vspace{-0.1em}
$p^q_j$ denotes the period of core j, and its formula is given by Eqn 5.31. Eqn 5.32 represents that each subchain finishes one full execution in $1/f_i$ periods of its core.

Eqns 5.33 and 5.35 describe the formulae for chains' throughput and latency (similar to \S\ref{sec:multicore}), and Eqns 5.36, 5.37 represent lower and upper bound constraints on these chain level metrics. We similarly can add constraints on node throughput using eqn 5.34. Note that the lower bound constraints are not tight here, i.e. $p_i \geq LT_x$ does not necessarily imply that the the subchain's period (eqn 5.32) will also be more than $LT_x$. This is mostly because geometric programming only supports less than constraints to maintain convexity.
